# Supplementary material for: Incorporating Posterior-Informed Approximation Errors into a Hierarchical Framework to Facilitate Out-of-the-Box MCMC Sampling for Geothermal Inverse Problems and Uncertainty Quantification
Source: arXiv:1810.04350 source file (2019-12-19)
Supplement: Supplementary file 1 [file si_wrr_2019_corner_reduced.pdf]

# Supporting Information for "Incorporating Posterior-Informed Approximation Errors into a Hierarchical Framework to Facilitate Out-of-the-Box MCMC Sampling for Geothermal Inverse Problems and Uncertainty Quantification"

Oliver J. Maclaren[1], Ruanui Nicholson[1], Elvar K. Bjarkason[1], John P. O'Sullivan[1] & Michael J. O'Sullivan[1]

[1]Department of Engineering Science, The University of Auckland, Auckland, New Zealand

**Contents of this file**

1. Figures S1 to S4

**Introduction:** In this supporting information we present the corner plots for both the synthetic slice model and the Kerinci test problem. Corner plots show both marginal and bivariate distributions for each rock type permeability.

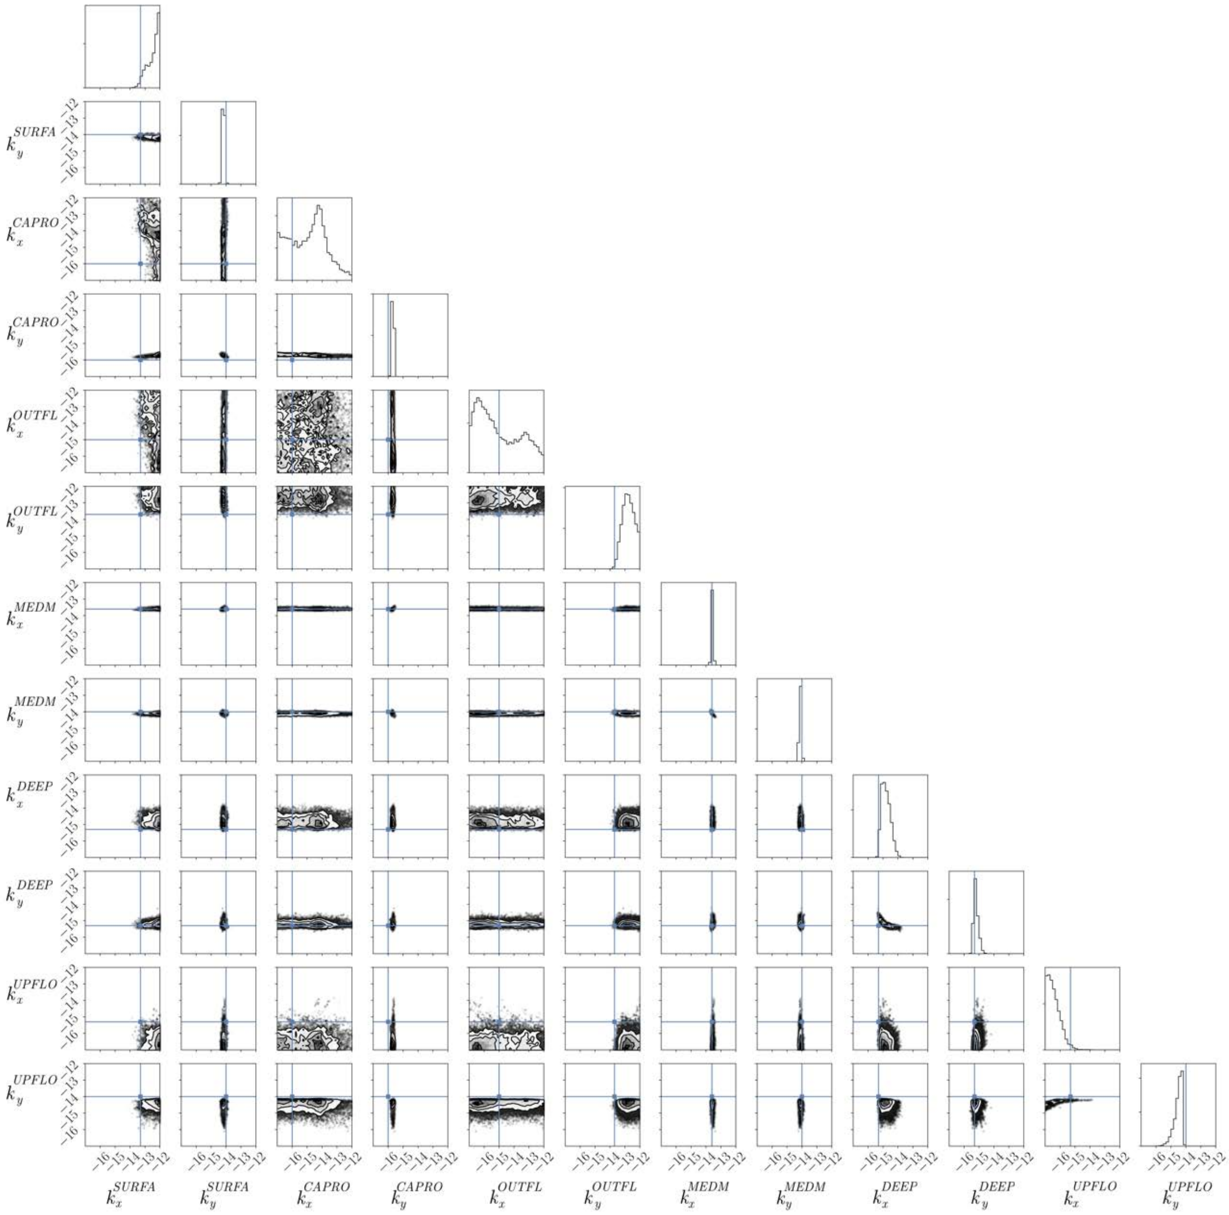


**Figure S1.** Corner plots for the synthetic case illustrating both marginal and bivariate distributions for rock permeabilities (log scale) under the naive, uncorrected model.

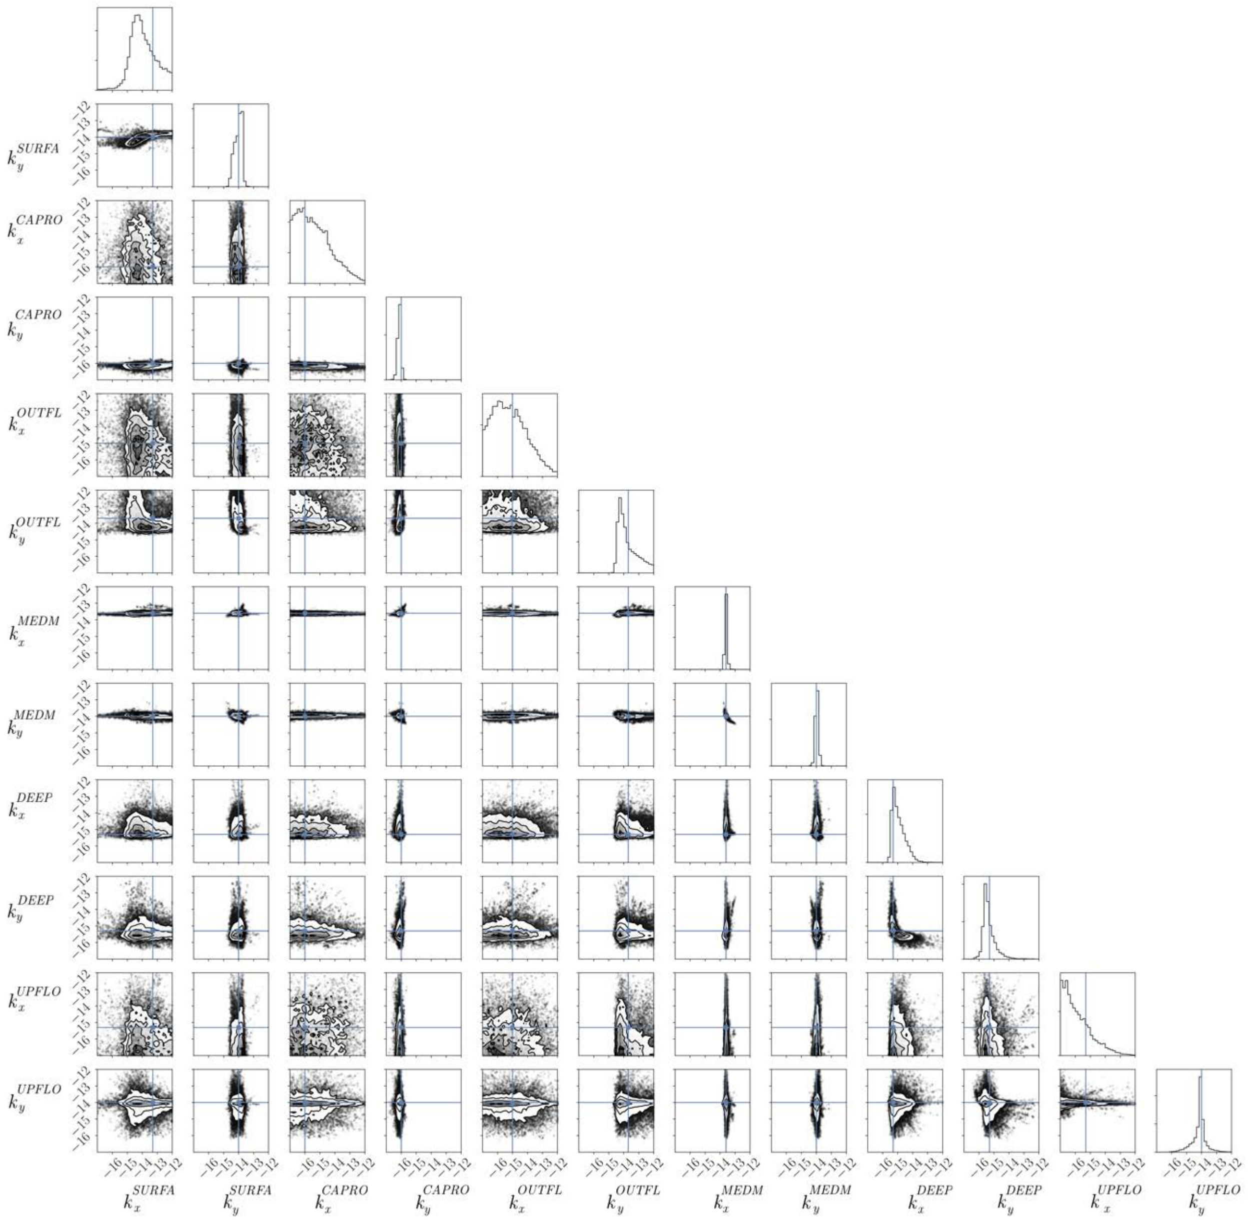


**Figure S2.** Corner plots for the synthetic case illustrating both marginal and bivariate distributions for rock permeabilities (log scale) incorporating the approximation errors.

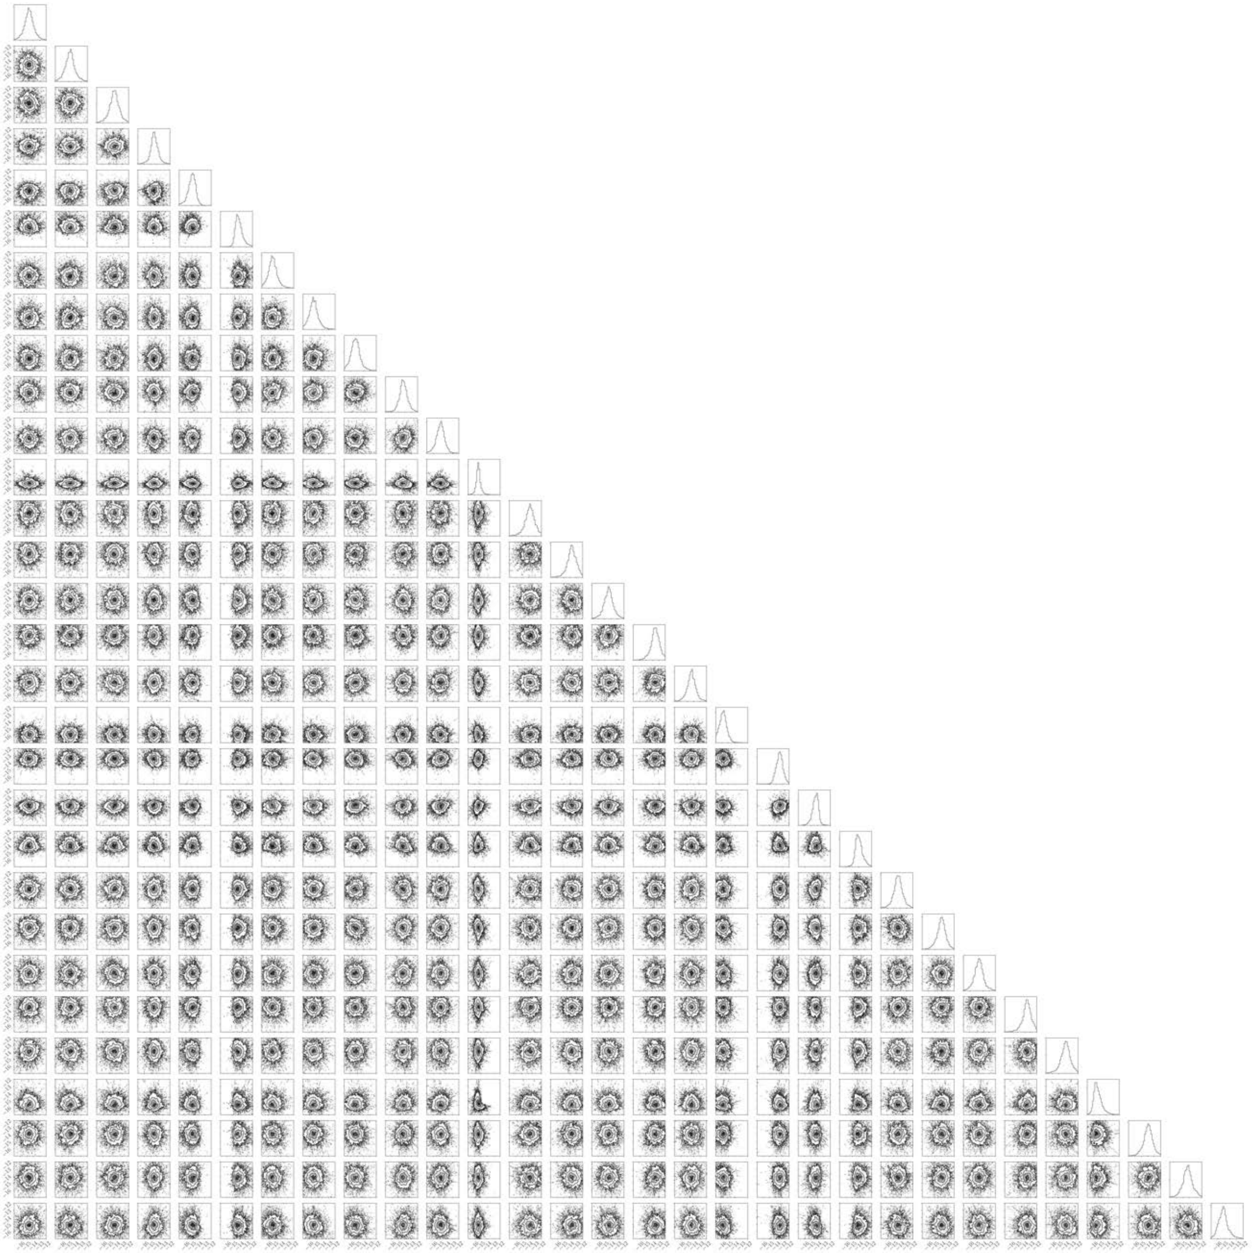

**Figure S3.** Corner plots for the Kerinci test case illustrating both marginal and bivariate distributions for rock permeabilities (log scale) under the naive, uncorrected model.

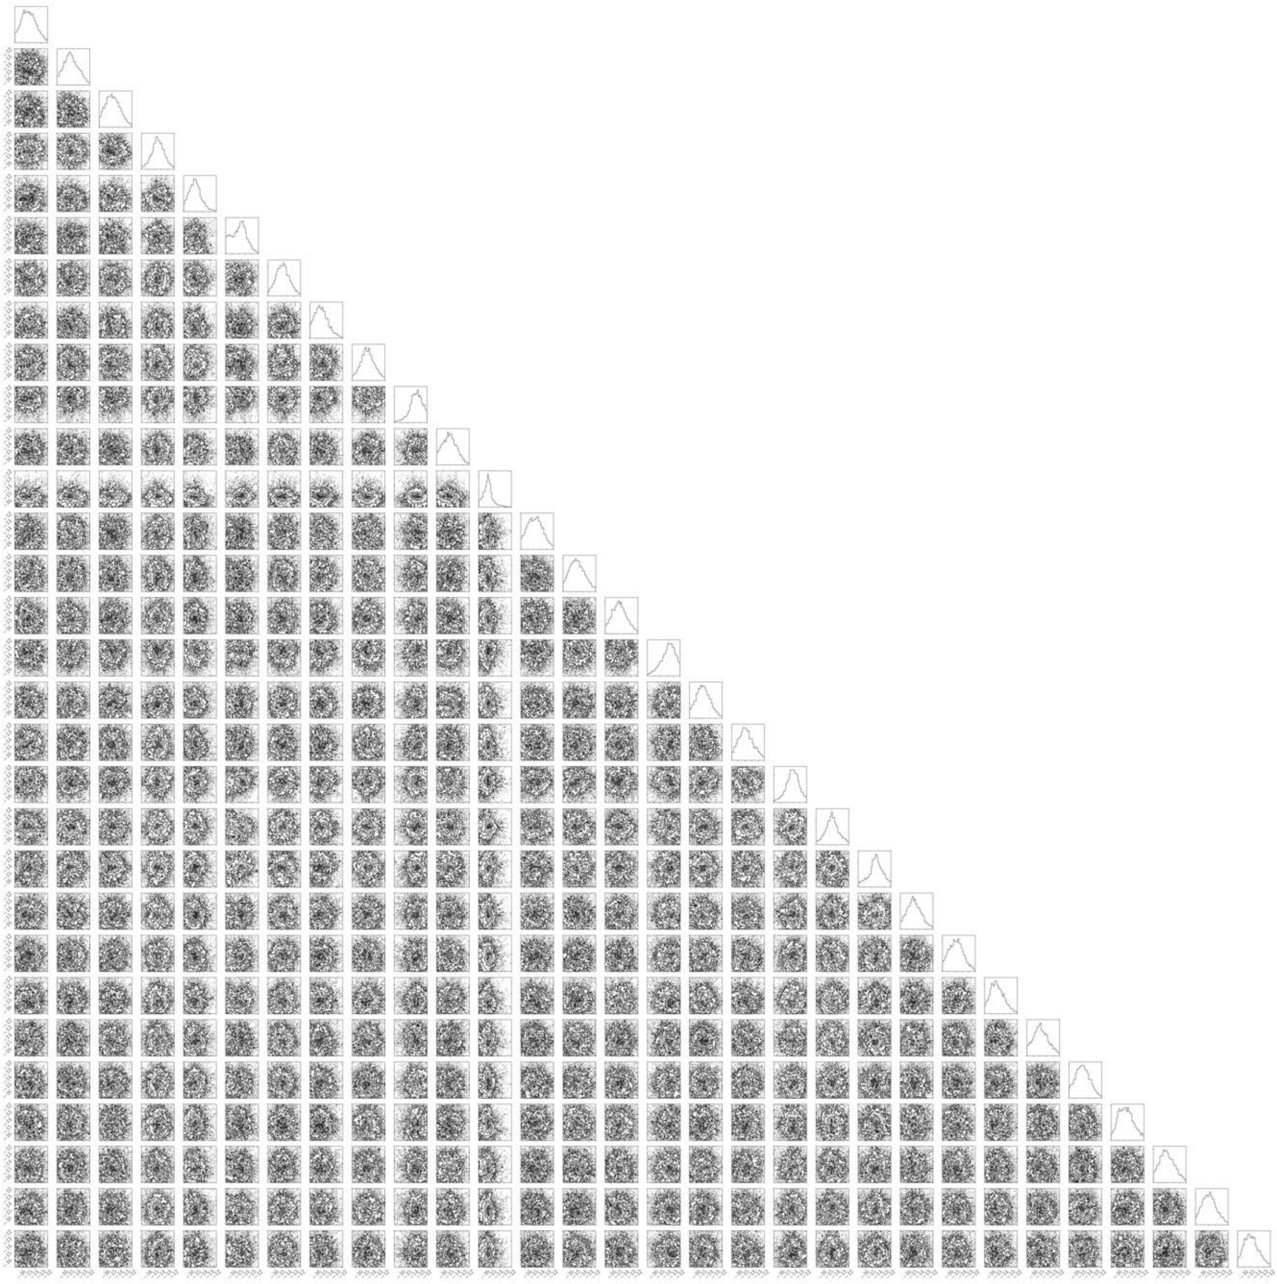

**Figure S4.** Corner plots illustrating both marginal and bivariate distributions for rock permeabilities (log scale) incorporating the approximation errors. All parameters are contained in the bulk of the support of the posterior.
